# Supplementary material for: T-TAMER: Provably Taming Trade-offs in ML Serving
Source: arXiv:2509.22992 source file (2026-08-03)
Supplement: Supplementary file 1 [file app_one_hyperbox.tex]

\section{Exact Optimization for Single-Line Constraints}\label{sec:1_hyperbox}

We now introduce the optimization approach for the Markovian Pandora’s box with \emph{single-line} constraints. This solution serves as a fundamental building block for our approach to the subsequent multi-line and forest settings.
% \jm{the transition from a graph with a line constraint to hyperboxes isn't super clear here. I think you want a line saying "A line constraint is equivalent to a graph with a hyperbox containing all nodes." or something.} \yy{No, we need more general use of this definition.}

\subsection{Algorithm for Line Constraints}\label{subsec:alg_1_hyperbox}

Before presenting details, we formally define a \textit{hyperbox} as a sequentially ordered set of boxes that form a \emph{directed path} within the original graph.

\begin{definition}[Hyperbox]\label{def:hyper} %\hf{Hyperbox for DAG seems weird...maybe only use it for multiple lines. } \yy{okk.}
Given an instance of the Markovian Pandora's box problem with $n$ boxes $\mathcal{B}$ associated with a directed acyclic graph (DAG) $G = (\mathcal{B}, E)$, a \emph{hyperbox} is a subset of boxes $\mathcal{H} := \{b_1, \ldots, b_n\} \subseteq \mathcal{B}$ such that the subgraph of $G$ induced by $\mathcal{H}$, denoted by $\mathcal{L}$, forms a directed path; that is, for each $i \in [n-1]$, the edge $(b_i, b_{i+1})$ belongs to $E$.
\end{definition}

Given a Markovian Pandora's box with a line constraint, we present our optimal solution for the one-line case (Alg.~\ref{alg:pd_1path}), which depends on the \textit{generalized reservation value} (Def.~\ref{def:GRV}) of a hyperbox. Specifically, our solution iteratively computes the GRV of the next box when exploring along a line. The process continues until the GRV of the next box falls below the current maximum reward, at which point the search terminates. 

\begin{algorithm}[!ht]\caption{Markov Pandora's Box, Single Line}\label{alg:pd_1path}
\begin{algorithmic}[1]
    \Require Ordered set of boxes $\{b_1,\ldots, b_n\}$, probing cost $\{c_1,\ldots, c_n\}$, GRV $\sigma_i(s)$ for all $i$, $x$ and $s$ (Alg.~\ref{alg:app:gw_1path}).
    \State Initialize $x \gets 0$, $i \gets 1$, $j \gets 1$, $\sigma \gets \sigma_i(0,0)$
    \While{$x < \sigma$} 
        \State Pay $c_i$ to open box $b_i$, observe reward/state $s^i$.
        \State $x \gets \max\{x, s^i\}$. \Comment{Update max reward}
        \State $\sigma \gets \sigma_{i+1}(s^i)$. \Comment{Look up the GRV}
        \State $i \gets i+1$.
    \EndWhile
    \State \textbf{Return} box $b_j$ that is opened and with the max reward.
\end{algorithmic} 
\end{algorithm}

%\jm{I'd use "maxval" or some other intuitive name instead of x} \yy{This notation needs to be aligned with the algorithm in the appendix. }

\subsection{Generalized Reservation Value (GRV)}\label{subsec:GRV}

We next show that probing according to the GRV maximizes the expected payoff. In the line case, all adaptive strategies are partially adaptive since the order constraint uniquely determines the probing sequence. Consequently, optimizing the strategy simplifies identifying the optimal adaptive stopping time. 

The optimal stopping time depends on the current state $(x, s^{i-1}, i)$, where $x$ is the highest observed reward, $s^{i-1}$ is the state of the last opened box $b_{i-1}$, and $i$ is the next box available for probing. For any state $(x, s^{i-1}, i)$ and strategy $\tau$, we denote $\tau(x, s^{i-1}, i)$ as the random stopping time conditioned on this state. We derive the equivalent reward given any stopping time $\tau$, as follows:

% \noindent We will use notation $s^i$ to denote the state that $b_i$ is at in the current run of the algorithm.\\

\begin{definition}[Equivalent Reward]\label{def:exp_reward}
    Given $\tau$ and $(x, s^{i-1}, i)$, we define the expected future reward following $\tau$, starting at state $(x, s^{i-1}, i)$, as
    \[\Phi^{\tau}(x, s^{i-1}, i) := \E [\max \{x , \max _{j=i} ^{\tau(x, s^{i-1}, i)}R_j\} - \sum_{j=i}^{\tau(x, s^{i-1}, i)} c_j]\]
    %\sandy{Why is this next paragraph in italics on the PDF?}\yy{Due to the definition environment....}
\noindent In addition, we use 
    \[
    \Phi (x, s^{i-1}, i)  = \Phi ^{\tau^*}(x, s^{i-1}, i)= \max _\tau \Phi^{\tau}(x, s^{i-1}, i) 
    \]
to denote the expected future reward following the optimal strategy $\tau^*$ starting at state $(x, s^{i-1}, i)$.
\end{definition}

 \noindent Given an optimal stopping time $\tau^*$, $\Phi$ can be solved inductively using Bellman’s principle of optimality~\cite{sbo98}: %\yy{added }\jm{Maybe one citation, or at least mentioning this is a well-known fact.}
  \begin{align*}
     & \Phi^{\tau^*}(x, s^{i-1},i) = \max \{x, -c_i + \quad \E[\max \{ \max\{x, s^i\}, \max_{j=i+1}^{\tau^*(x,s^i,i+1)} s^j - \sum_{j=i+1}^{\tau^*(x,s^i,i+1)} c_j \}] \} \\
     & = \max \{x, -c_i + \E_{s^i}[\phi^{\tau^*} (\max\{x,s^i\}, s^i, i+1) ]\}.
 \end{align*}
 %\hf{discuss a bit about this notation.}\yy{done.}
 % $\phi$ denote the expected future reward under the optimal stopping time, conditioned on the current maximum realized reward being $x$, the current state being $s^{i-1}$, and the next box to be considered being box $i$. 

Due to the optimality of the stopping rule over the remaining boxes, $\phi$ is given by the maximum of the expected utility between two options: (1) Stop at the current iteration (i.e., incur utility $x$); (2) Open the next box and then applying the optimal stopping strategy to the remaining boxes (i.e., the second term inside the max operator.)

Notice that for fixed $s^{i-1}$ and $i$, there exists a minimal $x$ such that the decision maker is \emph{indifferent} between stopping and opening the next box; that is, the two terms inside the max operator are equal. We define this quantity as the \emph{generalized reservation value} (GRV):

\begin{definition}[Generalized Reservation Value]\label{def:GRV}
	\label{def:grv}
	Given any state $(x, s^{i-1}, i)$, we define the generalized reservation value at the current state for box $b_i$, denoted by $\sigma_i$, as the smallest solution to: 
	\begin{equation}
	\E \Big[\Big( \max _{j=i} ^{\tau^*(\sigma_i, s^{i-1}, i)}R_j - \sigma_i\Big)_+ - \sum_{j=i}^{\tau^*(\sigma_i, s^{i-1}, i)} c_j\Big] = 0,
	\label{eq:grve}
	\end{equation}
    where $\tau^*$ is the optimal strategy.
\end{definition}

% \noindent Given current best reward $x$ and state $(x, s^{i-1}, i)$, the important quantity we care about is the difference $\Phi(x, s^{i-1}, i)-x$. This is the difference between expected future reward and current best reward. This quantifies the increase in payoff we can expect to get from continuing to explore optimally. We have the following definition: 
% \begin{definition}\label{def:add_reward}
%     Given state $(x, s^{i-1}, i)$, we define
%     \[H_i(x, s^{i-1}) = \Phi (x, s^{i-1}, i) - x\]   
% \end{definition}

% \noindent One immediate property of $H_i$ is that $H_i$ is non-negative since $\Phi (x, s^{i-1}, i) \ge x$ for any $x$. 

We conclude this section by presenting some GRV properties; see Appendix~\ref{sec:app:multi_line} for more details.
\begin{lemma}[Properties of GRV]\label{lem:properties_GRV}
 Given a Markovian Pandora's box with line precedence graph $\mathcal{L}=\left[b_1, \ldots, b_n\right]$, the generalized reservation value of every box $i \in [n]$ satisfies the following property. Given any state $s^{i-1}$:
 \squishlist
    \item $\sigma_i$ is independent of the current max reward $x$.
    \item $\sigma_i(s^{i-1}, i)$ is nondecreasing as additional boxes are appended to $\hyperb$.
    \item Let $\eta$ be the (random) index of the first box with a GRV smaller than $\sigma_i(s^{i-1}, i)$; then, $\sigma_i(s^{i-1}, i)$ depends only on the (sub)hyperbox $\hat{\hyperb} := \{b_i, \ldots, b_{\eta}\}$. If $i = \eta$ with probability $1$, then $\sigma_i(s^{i-1}, i)$ depends only on $b_i$. 
 \squishend

\end{lemma}

\subsection{Correctness and Running Time Analysis}\label{subsec:correct_time_line}

\noindent We first show the existence and uniqueness of the GRV.

\begin{theorem}[Optimality of GRV] \label{thm:unique_fair_cap}
The smallest solution to (\ref{eq:grve}) exists; hence, the generalized reservation value is well defined (Def.~\ref{def:grv}). Given the current state $(x, s^{i-1}, i)$ and $\sigma := \sigma_i(s^{i-1}, i)$: 

\squishlist
    \item If the generalized reservation value $\sigma > x$, all optimal stopping strategies proceed. 
    \item If $\sigma < x$, all optimal stopping strategies terminate.
    \item If $\sigma = x$, there exists an optimal stopping time $\tau^*(x, s^{i-1}, i) \geq i$.
\squishend

\end{theorem}

This theorem implies the correctness of our algorithm since it aligns with the optimal stopping time characterized above. Here, the optimal stopping time is indifferent to proceeding or stopping when the current max reward equals the GRV of the next box in line. To ensure the uniqueness of the optimal stopping time, WLOG, we adopt the convention that the optimal strategy $ \tau^*(\sigma_i, s^{i-1}, i) $ always stops at $ b_{i-1} $.  

Next, we introduce a lemma for efficiently computing the equivalent reward table for any given state, which is a key component of our algorithm to calculate the GRV. 

\begin{lemma}\label{lem:computing_rv}
    There is an efficient algorithm (Alg.~\ref{alg:app:gw_1path}) that computes $\phi (x,s, i)$ for all $i$, $x$ and $s$. 
\end{lemma}

Refer to Appendix~\ref{sec:app:details_exact_opt} for additional details. The proof's intuition is to first evaluate $\phi$ at the last box of the hyperbox and then backtrack to the first.

\noindent We can now present the main theorem of this section, i.e., that our algorithm can be implemented in polynomial time and maximizes the expected payoff. 

\begin{theorem}[Generalized Reservation Rule is Optimal for Single Hyperbox]\label{thm:GMR_path}
Algorithm \ref{alg:pd_1path} is optimal for the Markovian Pandora’s box problem in a single-line precedence graph
and can be computed in polynomial time and space.
\end{theorem}

\begin{proof}
The correctness follows from Thm~\ref{thm:unique_fair_cap}. 

For the running-time analysis, we first show that the reservation lookup can be done in polytime. Notice that $\hat{\sigma} := \sigma_i(s)$ satisfies that (1) for any $x > \hat{\sigma}$, $\phi (x, s, i) = x$ and (2) for any $x < \hat{\sigma}$, $\phi (x, s, i) \geq x$, we could do a binary search on the range of $x$ to recover the GRV. Since the $\phi$ table requires only polynomial time (Lem.~\ref{lem:computing_rv}), the overall running time is in polynomial. 

Regarding space use, storing the $\phi$ tables requires polynomial space. As the algorithm proceeds, it needs to store only the max reward. Thus, Algorithm \ref{alg:pd_1path} requires polynomial space. 
\end{proof}

 % Our objective is to show that Alg.~\ref{alg:pd_1path} maximizes the expected payoff $\Phi^{\tau}(0, 0, 0)$ (assume we are at state $0$ before the game starts).
